# Supplementary material for: Verifying LLM Inference to Detect Model Weight Exfiltration
Source: arXiv:2511.02620 source file (2026-03-12)
Supplement: Supplementary file 1 [file appendix-trusted-code-deployment.tex]

\section{Trusted Code Deployment: Concentrated Code Inspection} \label{sec:trusted-code-deployment}

We note that there are two ways that an attacker could exfiltrate data from the Inference Server:
\begin{enumerate}
\item \textbf{Unauthorized deployment}: The attacker bypasses the lab's standard deployment pipeline, e.g. leveraging an exploit in the deployment pipeline or by compromising the underlying hardware.
\item \textbf{Authorized deployment}: The attacker writes exfiltration code and deploys it using the lab's standard deployment pipeline—this code passes all pre-deployment tests, perhaps including manual review by several inference engineers.
\end{enumerate}

The possibility of \textit{authorized} deployments of exfiltration code poses a fundamental threat to Subsampled Output Verification, because it could lead to a situation in which the Verification Server independently reproduces inference outputs that exfiltrate model weights, yet doesn't flag these outputs as suspicious because they are consistent with the logged outputs. This suggests that the Verification Server will need to be provisioned with \textbf{trusted code}.

We note that the development of bug-free code is an extremely difficult problem, and we will not attempt to solve it in this work. Rather, we will propose a system for developing inference code that is \textbf{trusted by a diverse set of internal stakeholders}. Our system has two parts.

First, we propose a \textbf{release structure for inference code}. Inspired by semantic versioning, we suggest that each code version is identified as either a major version or a minor version, distinguished as follows:

\begin{itemize}
\item \textbf{Major versions}: This type of code is released only after it has undergone a stringent review process by a diverse set of internal stakeholders.
\item \textbf{Minor versions}: This type of code must pass a regression test checking that its output behavior does not exceed a ``\textit{divergence threshold}'' relative to the latest major version. This threshold parametrizes a tradeoff between security and development velocity.
\end{itemize}

\begin{figure}
    \centering
    \includegraphics[width=0.5\linewidth]{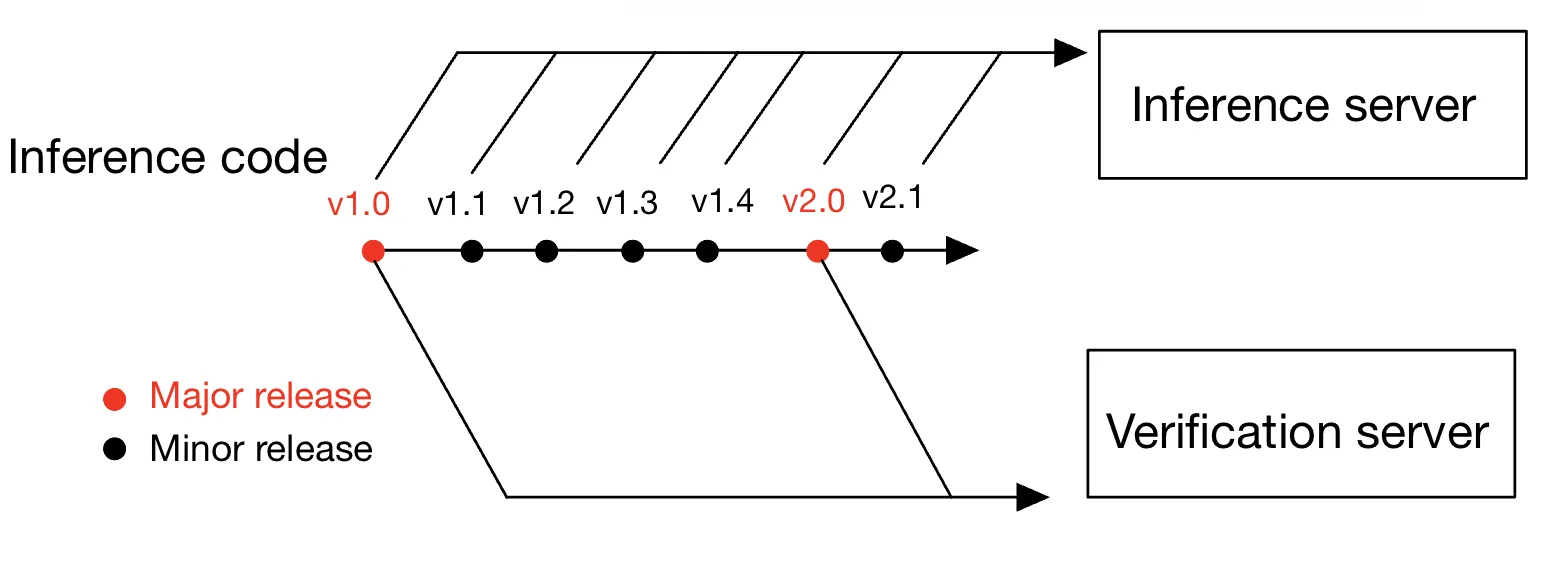}
    \caption{Enter Caption}
    \label{fig:enter-label}
\end{figure}

Secondly, we propose considering the inference team's ability to do code reviews as a limited resource, which we term ``auditing budget'' (e.g. engineering time for review, or number of different actors reviewing code). And then, applying a random application of auditing budget for each code review (outside of important reviews which always have a lot of attention). The goal here is to catch non-malicious code. This simple scheme is extremely powerful as it incentives all code-writers to act honestly, so long as they cannot predict if the auditing-budget will be applied upon them (this is based on the idea of the panopticon).

This scheme relies on the 1. while malicious code is difficult to catch, more attention makes it more likely to be caught, 2. code commits are signed by the author, and thus traceable back to someone (or something) that can be held responsible. From a utilitarian perspective, it is optimal for an adversary to behave honestly if the probability of being caught multiplied by the cost of being caught is sufficiently high. Some more work is needed to prove the game-theoretically optimal application of auditing budget.

\textbf{An auditing structure:}
\begin{enumerate}
\item Important code contributions/revisions are always reviewed, and use a large part of the auditing budget
\item Less-important code contributions (which still can introduce malicious code) are audited with random amounts of auditing budget.
\end{enumerate}
\begin{figure}
    \centering
    \includegraphics[width=0.5\linewidth]{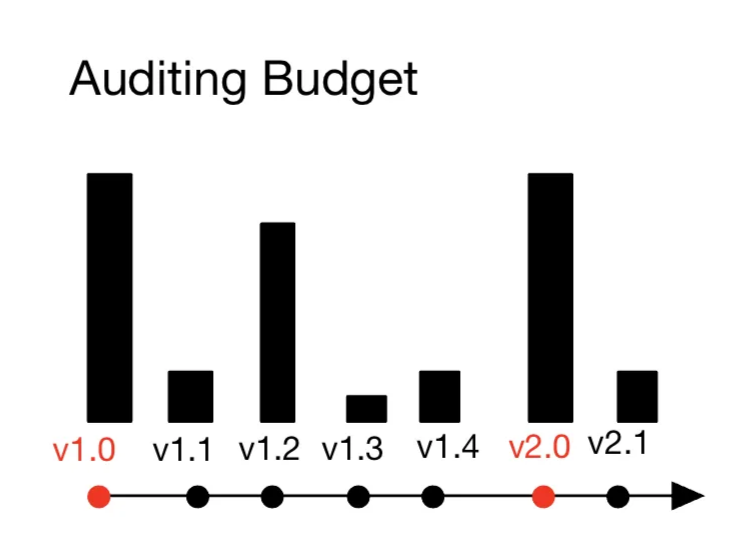}
    \caption{Enter Caption}
    \label{fig:enter-label}
\end{figure}
Thus, in this section, we have introduced a scheme to provision code for a verification server, by applying randomized code-review on a potentially untrusted codebase - addressing the unauthorized deployment problem.
